# Supplementary material for: UniGLM: Training One Unified Language Model for Text-Attributed Graph Embedding
Source: arXiv:2406.12052 source file (2024-12-23)
Supplement: Supplementary file 1 [file appendix.tex]

\section{More Experiment Details}
\noindent\textbf{Context Information.}\ \ We will inllustrate the concept of context information by taking ogbn-arxiv dataset as an examples.
\textbf{Domain information:} It is a paper from a citation network. All nodes in this citatation network represents a paper in Computer Science field.
\textbf{Node Status:} This node have 5 connected neighbors and the average degree of this citation network is 14.

\noindent\textbf{Datasets.}\ \ We evaluate the proposed UniGLM framework using seven publicly available TAG datasets. These datasets include one classic large-scale citation network Ogbn-Arxiv~\cite{hu2020open}, a co-purchase network Ogbn-Product from TAPE~\cite{he2024harnessing} and five E-commerce datasets extracted from Amazon~\cite{ni2019justifying}: Electronics-Computers (Computers), Books-History (History), Books-Children (Children), Sports-Fitness (Fitness), and Electronics-Photography (Photo). Noteblely, we use another co-purchase network from \cite{he2016ups} and \cite{mcauley2015image} named VideoGames. For node classification, we adhere to the standard data splits used in previous research for Ogbn-Arxiv, and Ogbn-Products, while we use a 5:20:75 split for the E-Commerce datasets. For link prediction, we adopt the widely used 5:10:85 split and sample equal number of negative links as positive links. 

\begin{table}[htbp]
\centering
 % 可选：减少行距
\setlength{\tabcolsep}{1pt} % 可选：减少列距
\small % 可选：减小字体
  \begin{tabular}{c|c|c|c|c|c}
   \hline
     Data &  Nodes & Edges & Ave Token &  Classes & Homophily Score\\
     \hline
     Ogbn-Arxiv & 169,343 & 1,166,243 & 235 & 40 & 0.6542 \\
     Ogbn-Products & 54,025 & 74,420 & 163.18 & 47 & 0.7950 \\
     Computers & 87,229 & 808,310 & 117 & 10 & 0.8503 \\
     History & 41,551 & 400,125 & 302 & 12 & 0.6975 \\
     Children & 76,875 & 1,631,453 & 280 & 27 & 0.4492 \\
     Fitness & 173,055 & 1,946,555 & 30 & 13 & 0.9092 \\
     Photo & 48,362 & 549,290 & 191 & 12 & 0.7712 \\
   \hline
\end{tabular}
\caption{Dataset statistics of eight TAGs.}
\label{dataset_stat}
\end{table}

\begin{itemize}
    \item \textbf{Ogbn-Arxiv~\cite{hu2020open}.} The Ogbn-Arxiv dataset is a directed graph, representing the citation network between all Computer Science(CS) arXiv papers. 
    \item \textbf{Ogbn-Products(subset)~\cite{he2024harnessing}.} The Ogbn-Products dataset represents an Amazon product co-purchasing network, with product decriptions as raw text.
    \item \textbf{Electronics-Computers(Computers)~\cite{ni2019justifying}.} The Electronics-Computers dataset is a segment of the Amazon co-purchase graph, where nodes represent goods, edges indicate that two goods are frequently bought together, node features are bag-of-words encoded product reviews by default, and class labels are given by the product category.    
    \item \textbf{Books-History(History)~\cite{ni2019justifying}.} Each node represents a book related to history domain, edges indicate that two books are frequently bought together and class labels are given by the book category.
    \item \textbf{Books-Children(Children)~\cite{ni2019justifying}.} Each node represents a book related to child domain, edges indicate that two books are frequently bought together and class labels are given by the book category.
    \item \textbf{Sports-Fitness(Fitness)~\cite{ni2019justifying}.} Each node represents a kind of item in the Sports and Fitness category.
    \item \textbf{Electronics-Photography(Photo)~\cite{ni2019justifying}.} This dataset contains review data from Amazon platform. Each node represents a review related to the item in the camera category.
\end{itemize}

\noindent\textbf{Baselines.}\ We compare UniGLM with five textual feature extraction methods. Previously we mentioned four methods including: SE, BERT, GIANT, PATTON. To comprehensively compare the proposed UniGLM with existing methods on multiple-datasets, we implement \textbf{MixGIA} as an additional baseline. MixGIA utilizes the GIANT framework and is applied to multiple datasets, leveraging the structural information of each dataset to fine-tune an a shared BERT model. Specifically, original GIANT construct a clustering tree to classify each node layer by layer. Our implementation of MixGIA set a fix number of layers for clustering tree and change the tree alone with the dataset per layer. 

\noindent\textbf{Experimental Settings.}\
Defaultly, UniGLM is trained on seven datasets and used as encoder for node textual attributes.
For node classification, we input UniGLM node embeddings into MLP and several different state-of-the-art GNN models and graph self-supervised learning methods, including GCN~\cite{mikolov2013efficient}, GraphSAGE~\cite{hamilton2017inductive}, RevGAT~\cite{li2021training}, GraphCL~\cite{you2020graph} and S2GAE~\cite{tan2023s2gae}. We run the experiments five times and report the mean result and standard deviation.  We use AUC, AP and Hit@100 as metrics for link prediction. We test with MLP. For the reproducibility of our experiments, we employ
GNN implementations from the PyG~\citep{fey2019fast} package. The default language model backbone is all-mpnet-base-v2 if not specified. Hyper-parameters are shown below.

\textbf{Transfer Learning Settings.} For \textbf{in-domain} transfer learning, we compare the performance of node classification and link prediction using node textual attributes encoded by a shallow embedding method (bag of words), BERT, Patton trained on Computers dataset as well as MixGIANT and UniGLM, both of which have been trained on seven datasets. For link prediction, co-view edges are used as the training set, while co-purchase edges are designated as the test set. For node classification, we randomly sample 5\% of the nodes as the training set, 20\% as the validation set, and use the remaining nodes as the test set. This process is repeated five times, and the average results are reported. For \textbf{cross-domain} transfer learning, we compare the performance of node classification under semi-supervised setting and few-shot setting using node textual attributes encoded by a shallow embedding method (bag of words), BERT, Patton trained on Computers dataset as well as MixGIANT and UniGLM, both of which have been trained on six datasets without ogbn-arxiv itself. Results of UniGraph is directly copied from the paper. We strictly follow the few-shot setting of UniGraph for evaluation.

\noindent\textbf{Hyperparameter}
Our hyperparameter for GNN is shown in Table \ref{table-gnn-hyper}.
\begin{table}[h!]
\centering
\begin{tabular}{lccc}
\hline
\textbf{Hyperparameters} & \textbf{GCN} & \textbf{SAGE} & \textbf{RevGAT} \\
\hline
\# layers & 3 & 3 & 3 \\
hidden dim & 256 & 256 & 256 \\
learning rate & 0.003 & 0.003 & 0.002 \\
dropout & 0.3 & 0.3 & 0.75 \\
epoch & 1000 & 1000 & 1000 \\
warmup epochs & 0 & 0 & 50 \\
early stop & 50 & 50 & 50 \\
\hline
\end{tabular}
\caption{Hyperparameters for GNN}
\label{table-gnn-hyper}
\end{table}

For UniGLM, we have hyperparameter in Table~\ref{Hyperparemeters} as follow:
\begin{table}[htbp!]
\centering
\small
\begin{tabular}{cc}
\toprule
Hyperparameters &  \\
\midrule \multirow{1}{*}{BATCH SIZE} &64 \\
\midrule \multirow{1}{*}{TEMPERATURE}   &0.3 \\
\midrule \multirow{1}{*}{NUM POS SAMPLES (t)}  &15 \\
\midrule \multirow{1}{*}{dropout}  &0.05 \\
\midrule \multirow{1}{*}{LEARNING RATE}  &2e-5 \\
\bottomrule
\end{tabular}
\caption{Hyperparemeters of UniGLM}
\label{Hyperparemeters}
\end{table}

\noindent\textbf{Device.} We compare the training and inference time cost of GIANT, PATTON and UGEmb. For GIANT and PATTON, the training time is the sum of training all eight TAGs listed above. For UniGLM, it is  the time to use all seven TAGs to train one model. Reported inference time is the time to encode Ogbn-Arxiv for each method. We use a A800(80G) for training and inference.

\newpage
\section{Learnable Positive Generation Scheme Analysis}
\textbf{Problem Setup}
Given:
\begin{itemize}
    \item \( \mathbf{E_c} \) as the central node embedding.
    \item \( \mathbf{E_s} = [\mathbf{e}_1, \mathbf{e}_2, \dots, \mathbf{e}_k] \) as the embeddings of positive samples.
    \item \( \mathbf{w} = [w_1, w_2, \dots, w_k] \) as the corresponding weights.
\end{itemize}

\textbf{Final Formulas}

\begin{enumerate}
    \item \textbf{First Approach: Weighted Embeddings Before Similarity}
    \[
    \text{similarity}_1 = \frac{\mathbf{E_c} \cdot \left(\sum_{i=1}^{k} w_i \mathbf{e}_i\right)}{\|\mathbf{E_c}\| \sqrt{\sum_{i=1}^{k} \sum_{j=1}^{k} w_i w_j (\mathbf{e}_i \cdot \mathbf{e}_j)}}
    \]

    \item \textbf{Second Approach: Weighted Similarity After Computation}
    \[
    \text{similarity}_2 = \frac{1}{\|\mathbf{E_c}\|} \sum_{i=1}^{k} \frac{w_i (\mathbf{E_c} \cdot \mathbf{e}_i)}{\|\mathbf{e}_i\|}
    \]
\end{enumerate}

\textbf{Analysis}

\begin{itemize}
    \item \textbf{First Approach:} In the first approach, we first aggregate the positive sample embeddings using the weights, resulting in a single weighted sum vector. The similarity between this aggregated vector and the central node embedding \( \mathbf{E_c} \) is then computed. This method effectively smooths out individual variations among the samples, potentially reducing the impact of outliers or noisy samples.
  
    \item \textbf{Second Approach:} In the second approach, the cosine similarity between \( \mathbf{E_c} \) and each sample embedding \( \mathbf{e}_i \) is calculated individually, weighted by \( w_i \), and then summed. This method allows the influence of each sample to be more direct and individual, but it can make the final similarity score more sensitive to noise or outliers, especially if the corresponding weight is high.
\end{itemize}

\textbf{Conclusion}

\begin{itemize}
    \item \textbf{First Approach:} Tends to produce a more robust and stable similarity measure, as it reduces the influence of outliers by aggregating embeddings first.
    \item \textbf{Second Approach:} May lead to less robust results, as individual noisy or irrelevant samples with high weights can disproportionately affect the final similarity score.
\end{itemize}

\section{More Experiments Results}
This table~\ref{table-nc-appendix} is the other half of node classification results.
Figure~\ref{fig-lp-hit} is the results for link prediction task.

\begin{figure}[h!]
    \centering
    \includegraphics[width=0.8\linewidth]{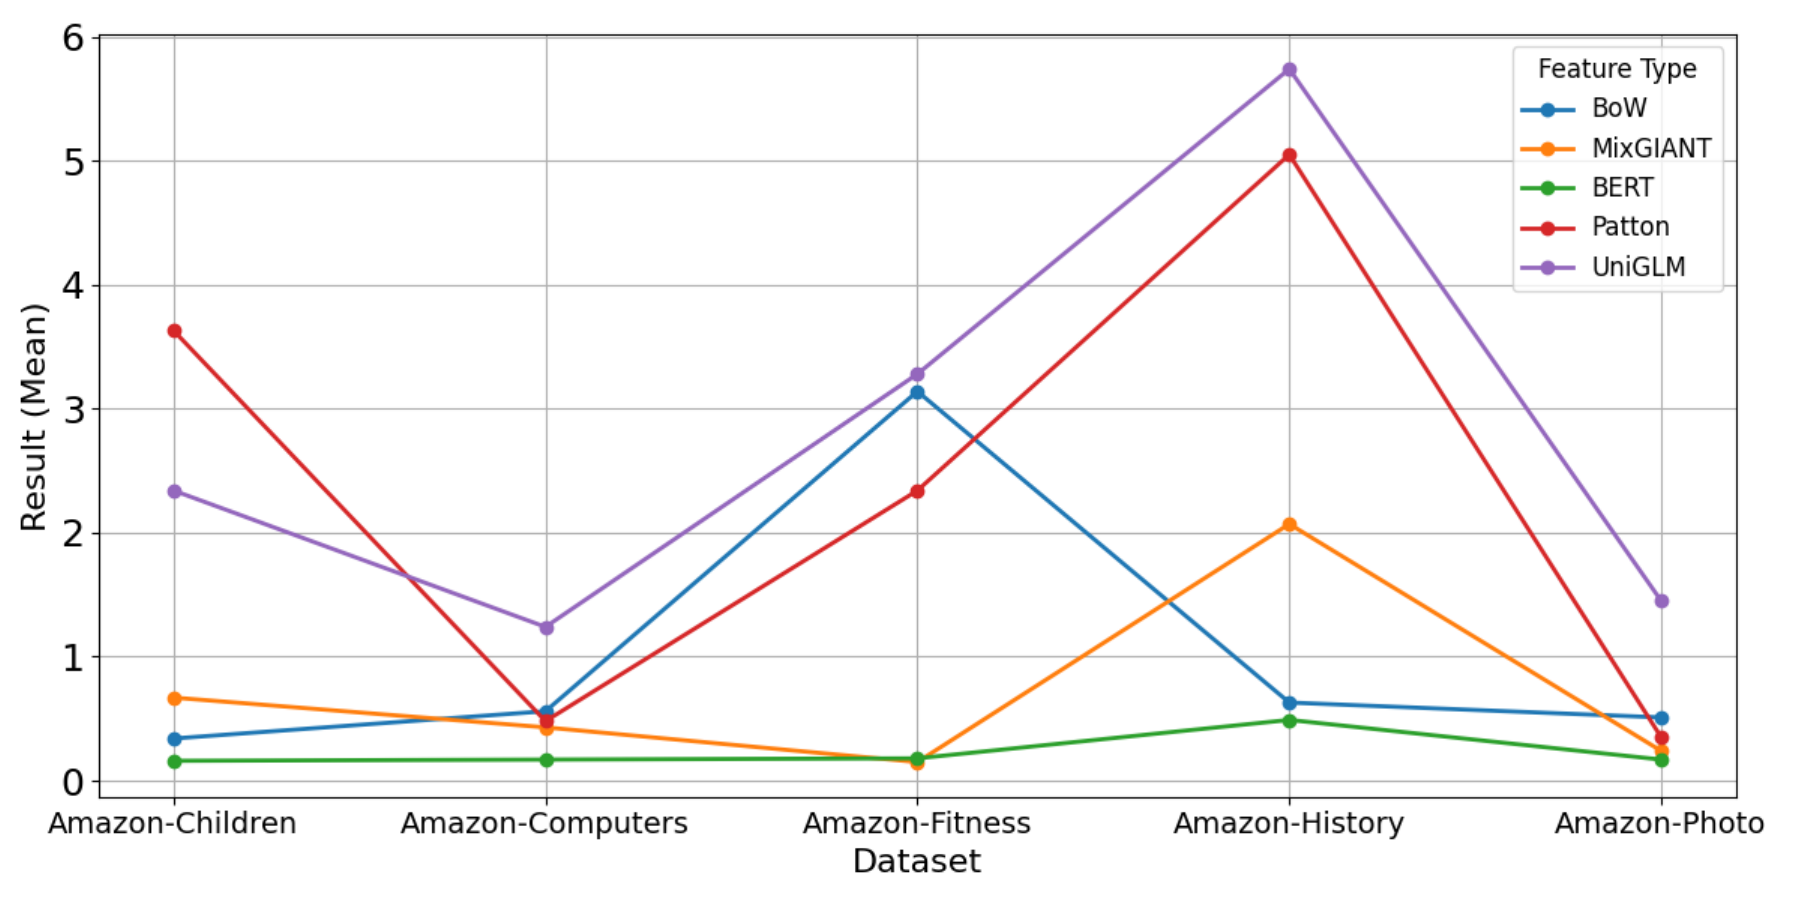}
    \caption{Link Prediction Results in Hit@100 metric.}
    \label{fig-lp-hit}
\end{figure}

\begin{table*}[h!]
\centering
\resizebox{\textwidth}{!}{
\begin{tabular}{c|c|c|c|c|c} 
\toprule
\midrule
Dataset                    & Emb Types  & MLP                            & GCN                            & SAGE                           & RevGAT                             \\ 
\midrule
\multirow{6}{*}{History} & SE & 73.19±0.36 (+14.36\%)& 77.03±0.70 (+7.06\%)& 77.63±0.22 (+7.72\%)& 77.83±0.27(+7.08\%)\\
 & BERT & 78.79±0.31 (+6.23\%)& 80.33±0.33 (+2.66\%)& 80.63±0.33 (+3.71\%)& 80.69±0.22(+3.28\%)\\
 & GIANT & 81.37±0.32 (+2.86\%)& 80.88±0.19 (+1.97\%)& 82.25±0.19 (+1.67\%)& 81.70±0.26(+2.01\%)\\
 & PATTON & \underline{82.88±0.24 (+0.99\%)}& \textbf{82.41±0.20 (+0.07\%)}& \textbf{83.43±0.18 (+0.23\%)}& \textbf{82.94±0.07(+0.48\%)}\\
 & MixGIA & 81.18±0.24 (+3.10\%)& 81.83±0.19 (+0.78\%)& 82.38±0.19 (+1.51\%)& 81.94±0.23(+1.71\%)\\
 & UniGLM & \textbf{83.70±0.10} & \textbf{82.47±0.30} & \textbf{83.62±0.14} & \textbf{83.34 ± 0.24}\\
\midrule
\multirow{6}{*}{Fitness} & SE & 78.07±0.18 (+15.81\%) & 83.20±0.19 (+9.22\%) & 83.65±0.17 (+9.17\%) & 84.26±0.16(+7.83\%)\\
 & BERT & 74.92±0.26 (+20.68\%) & 80.77±0.23 (+12.50\%) & 81.29±0.19 (+12.34\%) & 80.96±0.49(+12.23\%)\\
 & GIANT & 89.03±0.07 (+1.55\%) & 89.63±0.14 (+1.38\%) & 90.15±0.06 (+1.30\%) & 90.28±0.10(+0.64\%)\\
 & PATTON & \underline{89.60±0.22 (+0.90\%)}& \underline{90.03±0.21 (+0.93\%)}& \underline{90.61±0.12 (+0.78\%)}& \textbf{90.58±0.22(+0.31\%) }\\
 & MixGIA & 85.49±0.25 (+5.76\%) & 87.89±0.14 (+3.39\%) & 87.77±0.11 (+4.04\%) & 87.51±0.23(+3.83\%)\\
 & UniGLM & \textbf{90.41±0.14} & \textbf{90.87±0.14} & \textbf{91.32±0.07} & \textbf{90.86±0.09}\\
 \midrule
\multirow{6}{*}{Children} & SE & 38.84±0.35 (+34.81\%) & 43.19±0.31 (+17.11\%) & 44.83±0.24 (+17.09\%) & 43.00±0.18(+19.56\%)\\
 & BERT & 44.00±0.83 (+19.00\%) & 46.88±0.60 (+7.89\%) & 47.97±0.55 (+9.42\%) & 48.00±0.11(+7.10\%)\\
 & GIANT & 48.95±0.23 (+6.97\%) & 48.47±0.35 (+4.35\%) & 51.41±0.42 (+2.10\%) & 50.63±0.36(+1.54\%)\\
 & PATTON & \underline{49.91±0.13(+4.91\%)}& \underline{49.98±0.38 (+1.20\%)}& \underline{52.01±0.50(+0.92\%)}& \underline{51.07±0.21(+0.67\%)}\\
 & MixGIA & 48.17±0.32 (+8.70\%) & 49.55±0.21 (+2.08\%) & 50.11±0.39 (+4.75\%) & 49.29±0.27(+4.30\%)\\
 & UniGLM & \textbf{52.36±0.26} & \textbf{50.58±0.26} & \textbf{52.49±0.21} & \textbf{51.41 ± 0.34}\\
\midrule
\multirow{6}{*}{Photo} & SE & 61.24±0.41 (+27.82\%) & 71.70±0.16 (+11.91\%) & 72.14±0.33 (+13.00\%) & 71.63±0.23(+13.05\%)\\
 & BERT & 60.03±0.14 (+30.40\%) & 69.63±0.42 (+15.24\%) & 70.25±0.36 (+16.04\%) & 68.79±0.09(+17.72\%)\\
 & GIANT & \underline{77.43±0.27 (+1.10\%)}& \underline{79.79±0.14(+0.56\%)}& \underline{81.17±0.23 (+0.43\%)}& \textbf{80.69±0.43(+0.36\%)}\\
 & PATTON & 74.97±0.43 (+4.42\%) & 78.40±0.18 (+2.35\%) & 78.79±0.01 (+3.46\%) & 79.79±0.14(+1.49\%)\\
 & MixGIA & 72.17±0.30 (+8.47\%) & 77.06±0.14 (+4.13\%) & 77.68±0.21 (+4.94\%) & 77.68±0.39(+4.25\%)\\
 & UniGLM & \textbf{78.28±0.11} & \textbf{80.24±0.10} & \textbf{81.52±0.17} & \textbf{80.98±0.34}\\
\midrule
\bottomrule
\end{tabular}
}
\caption{Semi-supervised accuracy results on MLP and state-of-art GNNs with various embeddings for Children, Computers, History, PubMed, and Ogbn-Arxiv datasets. More results can be seen in Appendix.}
\label{table-nc-appendix}
\end{table*}

\begin{table}
\centering
\begin{tabular}{c|c|c|c|c} 
\toprule
Dataset                  & Emb Types & Photo      & History    & Products  \\ 
\midrule
\multirow{5}{*}{S2GAE}   & SE        & 84.06±0.19 & 47.05±0.27 & 89.93±0.09     \\ 
\cmidrule{2-5}
                         & BERT      & 83.64±0.09 & 48.70±0.40 & 88.22±0.07     \\ 
\cmidrule{2-5}
                         & GIA       & 85.15±0.13 & 50.72±0.10 & 90.66±0.09     \\ 
\cmidrule{2-5}
                         & PATTON    & 85.19±0.18 & 48.60±0.41 & 90.73±0.09     \\ 
\cmidrule{2-5}
                         & UniGLM    & \textbf{85.23±0.11} & \textbf{51.42±0.10} & \textbf{91.30±0.10}     \\
\bottomrule
\end{tabular}
\caption{Semi-supervised accuracy results on state-of-art graph self-supervised learning S2GAE with various embeddings for Photo, Children, History, Ogbn-Products, and Fitness datasets.}
\label{table-nc-gssl}
\end{table}
